# Supplementary material for: On The Expressivity of Objective-Specification Formalisms in Reinforcement Learning
Source: arXiv:2310.11840 source file (2024-02-17)
Supplement: Supplementary file 1 [file app-definititions.tex]

\section{Appendix: Definitions}

\begin{definition}
    
\end{definition}
